# Supplementary material for: Comparative Study of First and Second Switches with Nearly Identical Switching Current in Bi$_2$Sr$_2$Ca$_{0.85}$Y$_{0.15}$Cu$_2$O$_y$ Intrinsic Josephson Junctions
Source: arXiv:1909.06101 source file (2019-09-13)
Supplement: Supplementary file 1 [file Supple_Mater.pdf]

# Supplementary Material of
# "Comparative Study of First and Second Switches with Nearly Identical Switching Current in $Bi_2Sr_2Ca_{0.85}Y_{0.15}Cu_2O_y$ Intrinsic Josephson Junctions"

Ayami Yamaguchi, Haruka Ohnuma, Yuji Watabe, Shumpei Umegai, Kazutaka Hosaka, and Haruhisa Kitano*

*e-mail: hkitano@phys.aoyama.ac.jp

## 1. How to distinguish the switches in IJJs

In the measurements of the switching current density of Josephson junctions, by applying a bias current with a constant rate, the current where the drastic increase of voltage across the junction is repeatedly recorded. Since the IJJs have several junctions, the measured voltage is increased in a step-by-step manner for every switching event, as shown in Fig. S1. In this work, we set the appropriate threshold value for each switch and monitored both voltages just before and after the phase switch. Thus, we can clearly distinguish between the switches from the zero-voltage state to the first voltage state and those from the 1st to the 2nd voltage state. Even if the switching current between the 1st and 2nd SWs is almost the same, we can distinguish them, because of the different voltages, as shown in Fig. S1(b).

In the high-quality IJJs including several junctions with nearly equivalent properties, the measured distribution does not always consist of the phase switches arising from the identical junction. The fitting analyses of the switching rate as a function of bias current are useful to verify the components included in the measured distribution and to extract the main contribution, as was described in Ref. [12] of the main text. In this work, as shown in Fig. 2 of the main text, we confirmed that the 1st SW included only a single component derived from the events in the identical junction (J1). The main contribution to the 2nd SW was attributed to the events occurring in another junction (J2), which was distinguishable from J1 at least down to 2 K.

If IJJs have two junctions with completely equivalent properties, it will be quite difficult to distinguish them by using the present model based on a single Josephson junction. However, in such an ideal case, the two junctions are expected to be frequently switched at the same time, which can be distinguished in our measurements.

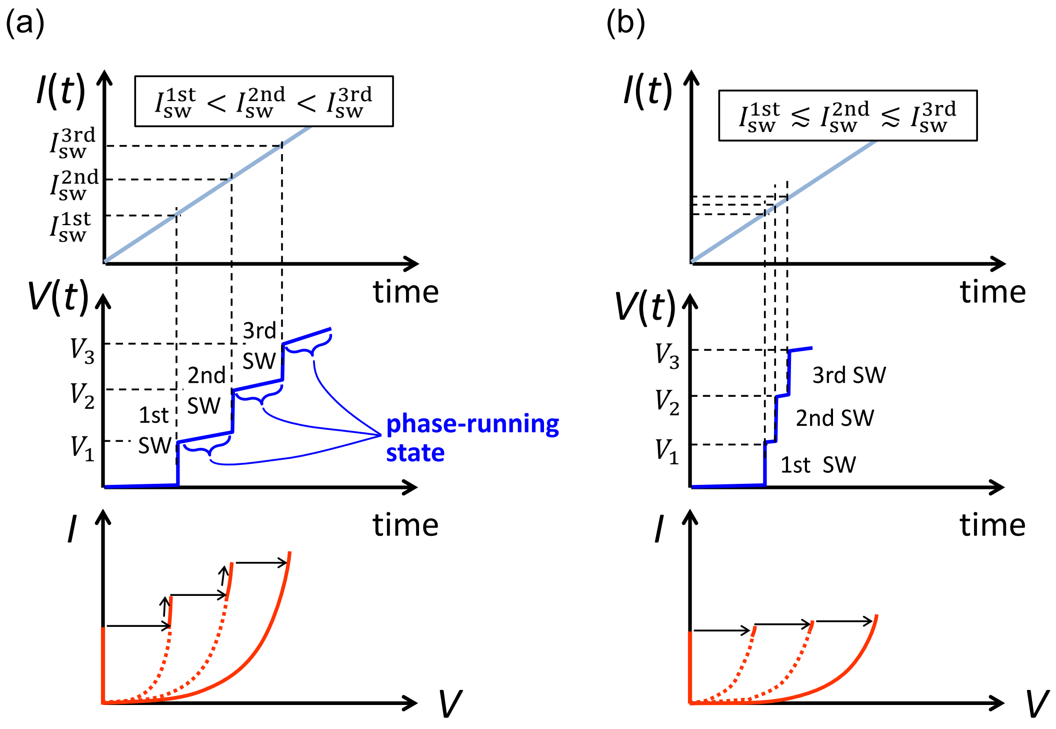


**Fig. S1.** (Color online) Schematics of waveforms for the current biasing IJJs with a constant rate, the voltage across the IJJs, and the resultant current-voltage characteristics. (a) the case of IJJs with different switching current, which is typical in the previous studies, and (b) the case of IJJs with almost the same switching currents, as like this work.

## 2. Positional relationship between the junctions measured in the 1st and 2nd SWs

When the phase switches in the bridge-type IJJs are detected by using the method described in the previous section, it is very difficult to determine a position of the switched junction and a positional relationship between the switched junctions. This shows a sharp contrast to the switches in the mesa-type IJJs, where the 1st SWs are considered to occur at a surface junction in the nearest neighborhood of the normal electrode. In order to specify the switched junctions in the bridge-type IJJs, the precise fabrication of IJJs with only a few junctions and the careful measurements of the switching current distribution for each order of SWs are required. Unfortunately, such a measurement has not been reported yet, as far as we know. Nevertheless, in this work, we consider that the two junctions (J1 and J2) measured in the 1st and 2nd SWs are very closely located, as we will show below.

There are two reasons in the above consideration. The first reason is that the effect of ac Josephson current occurring after the 1st SW, which is a main issue of this work, only concerns a closely-located junction in the IJJs with thin superconducting layers. If J2 is far from J1, all of intervening junctions must remain in the zero-voltage state. This is effectively equivalent to a situation that a thick superconducting layer is inserted between J1 and J2. This

suggests that the ac Josephson current occurring in J1 cannot affect J2, since it is well screened by the thick superconducting layer, as like an artificial array of the conventional Josephson junctions. In other words, the electromagnetic radiation due to ac Josephson current after the 1st SW can capacitively activate another junction only through a poor screening in the thin superconducting layers of IJJs. Such a capacitive coupling is expected to be moderately damped across the thin superconducting layers, suggesting the stronger coupling between the junctions located more closely.

The second reason is found in the measured current-voltage characteristics, as shown in Fig. S2. If J1 and J2 are spatially separated and the critical current for them is enough smaller than that for the intervening junctions, J2 can be independently switched without any influence from J1. In such a case, a larger switching current, corresponding to the higher order SWs than the 2nd SW, should be observed in the current-voltage characteristics, showing a contrast to the results in Fig. S2. Thus, we conclude that J1 and J2 studied in this work are probably adjacent.

On the other hand, our previous studies suggested that the second junction was not always adjacent to the first junction, since the switching current for the 2nd SW is larger than that for the 1st SW. Even in those cases, the second junction is considered to be located in the neighborhood of the first junction (For instance, the second-neighbor position or the third-neighbor position), because of the first reason mentioned above.

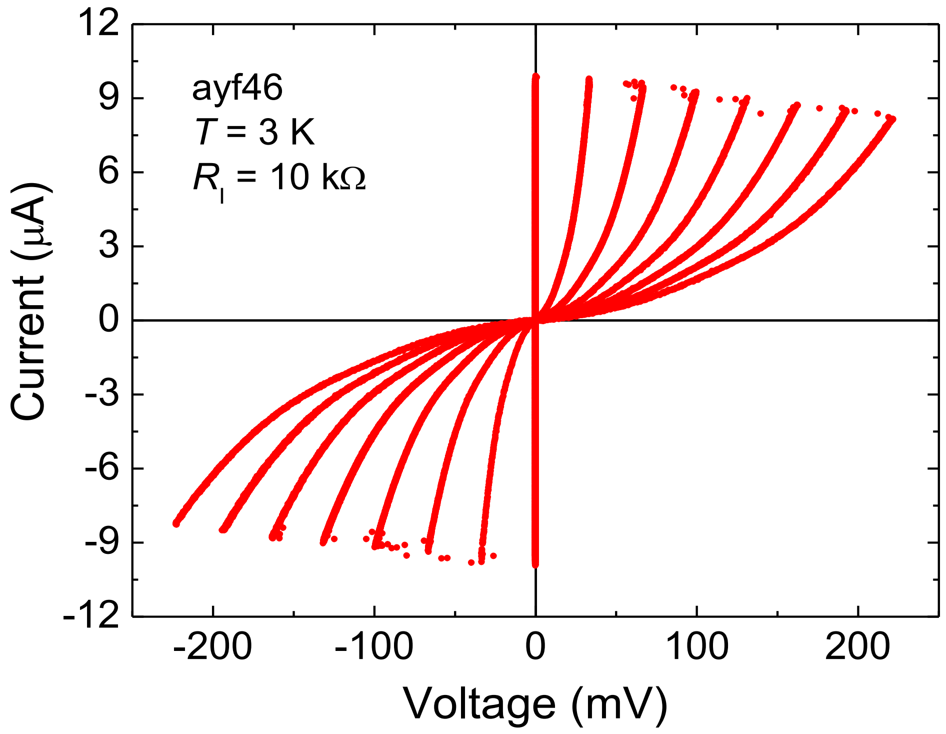


**Fig. S2.** (Color online) Typical current-voltage characteristics of the measured IJJs.
